# Supplementary material for: Did I delete my cookies? Cookies respawning with browser fingerprinting
Source: arXiv:2105.04381 source file (2021-05-07)
Supplement: Supplementary file 1 [file appendix3.tex]

\section{Appendix}

\begin{figure}[!ht]
    \centering
        \hspace*{-.8cm}%

    \includegraphics[width=.5\textwidth]{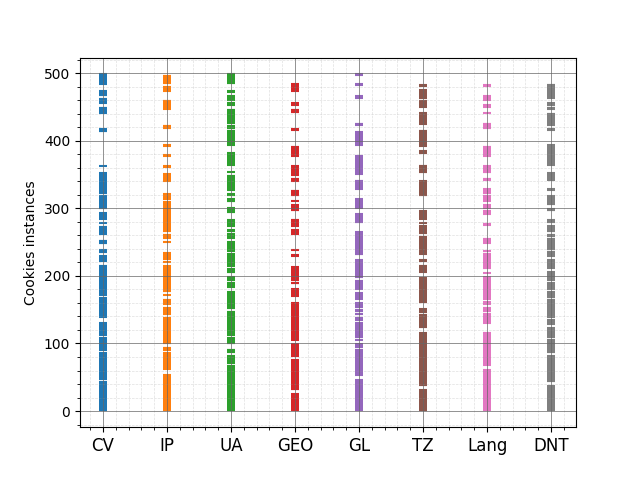}
    \caption{Features used with the top 500 cookies. \normalfont{The cookies ranking is based on the number of features used. \textit{For every cookie instance, we mark the set of features used to respawn the cookie. 
    CV: Canvas. IP: IP address. UA: User agent. GEO: Geolocation.  GL: WebGL. TZ: time zone.  Lang: Accept language. DNT: Do not track}}}
    \label{fig:feature500}
\end{figure}

\subsection{Additional results}

\subsubsection{HttpOnly feature analysis}

HttpOnly feature is used to specify if the cookie can be accessed through client side scripts or not. An HttpOnly cookie can only be accessed through HTTPS.
A cookie accessible from browser side through scripts is the subject of Cross-site Scripting (XSS) attack.
If the tracker manage to inject the script in the user's browser, he can have access and read the non http only cookies. 
Using the HttpOnly feature, we prohibit the usage of the cookies from the client side,
hence, even if the attacker manage to inject a script on the client side he will not be able to access her cookies.\\

\begin{figure}[!htbp]
    \centering
    \includegraphics[width=0.5\textwidth]{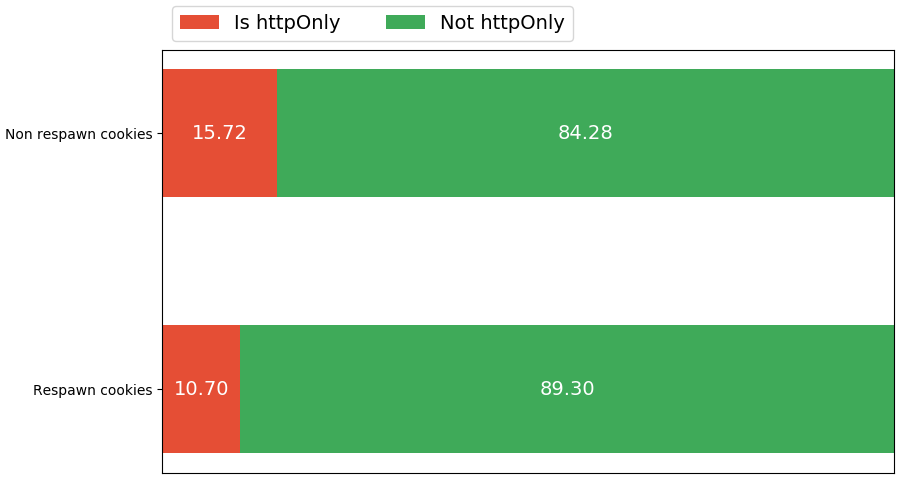}
    \caption{Percentage of usage of httpOnly attribute in respawned and non respawned cookies. }
    \label{fig:httponly}
\end{figure}

Figure \ref{fig:httponly} presents the percent of adoption of httpOnly for \textit{non respawn} cookies compared to \textit{respawn cookies}.
We notice that only 10.70\% of respawn cookies are httpOnly compared to 15.72\% of non respawn cookies.

\paragraph{Respawn cookies keys analysis}
We present  the keys of the respawned cookies (Figure \ref{fig:names})

\begin{figure}[!ht]
    \centering
    \includegraphics[width=0.5\textwidth]{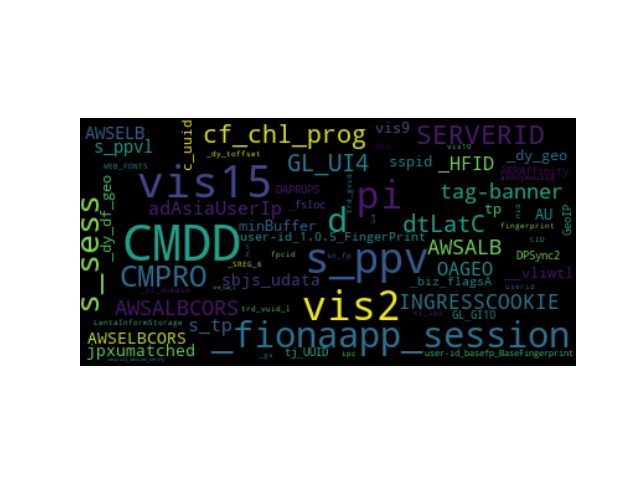}
    \caption{Keys of the respawned cookies  }
    \label{fig:names}
\end{figure}

  \begin{figure}[htbp]
    \centering
\subfloat{\includegraphics[width=0.4\textwidth]{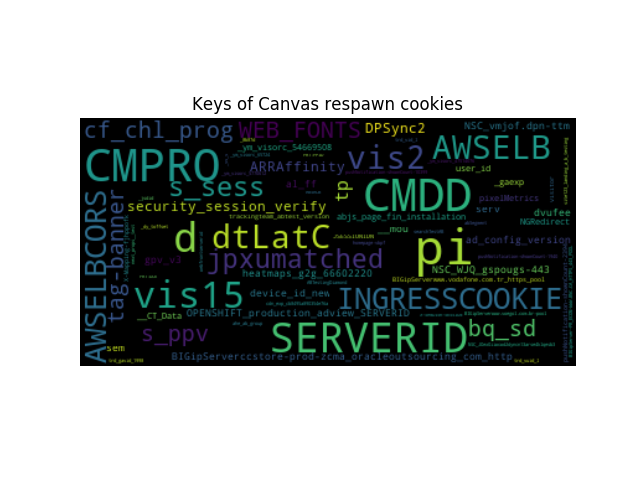}\label{fig:canvas}}
\hfil
\subfloat{\includegraphics[width=0.4\textwidth]{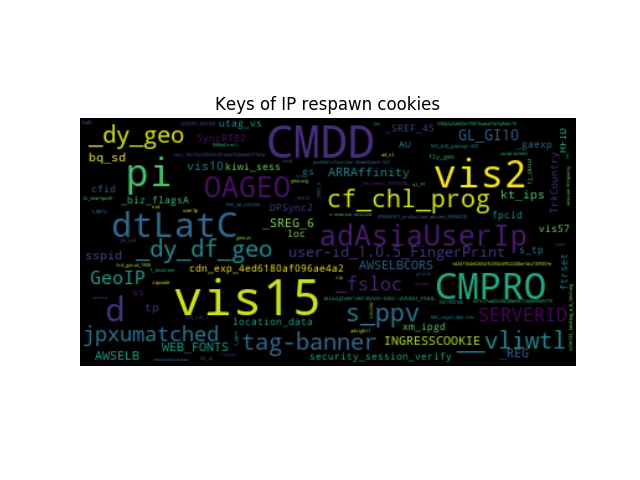}\label{fig:b}}

\medskip
\subfloat{\includegraphics[width=0.4\textwidth]{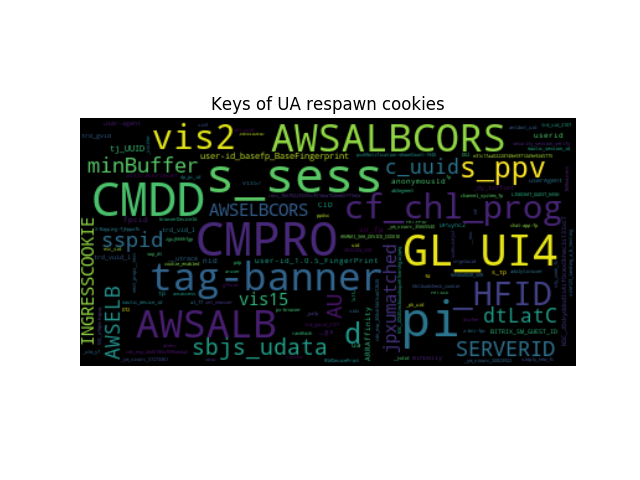}\label{fig:c}}
\hfil
\subfloat{\includegraphics[width=0.4\textwidth]{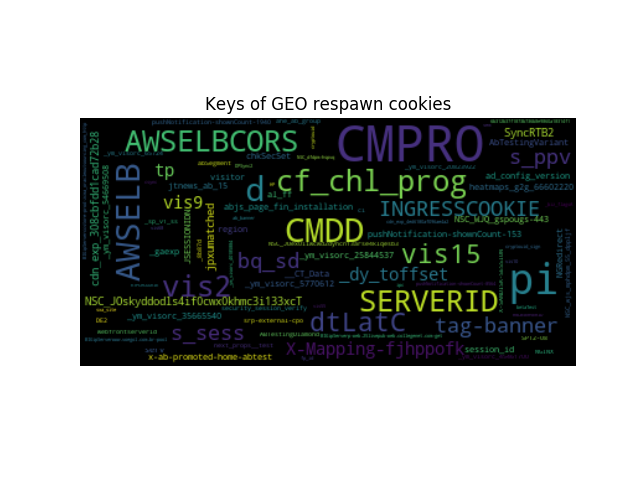}\label{fig:d}}

\medskip
\subfloat{\includegraphics[width=0.4\textwidth]{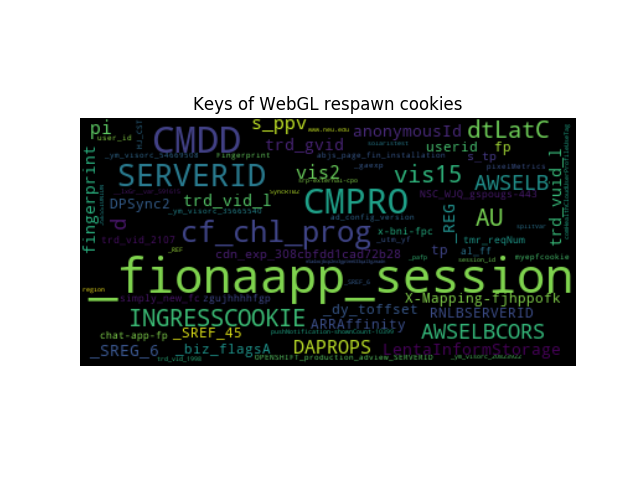}\label{fig:e}}
\hfil
\subfloat{\includegraphics[width=0.4\textwidth]{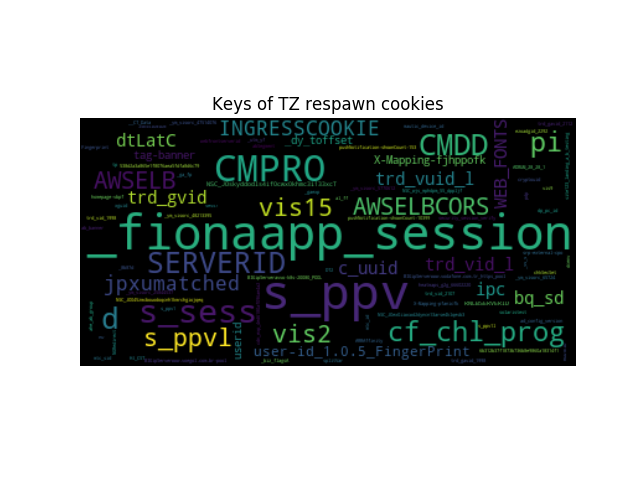}\label{fig:f}}

\medskip
\subfloat{\includegraphics[width=0.4\textwidth]{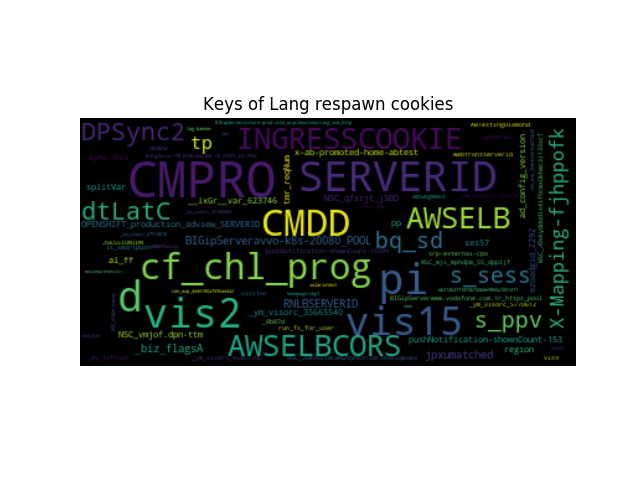}\label{fig:g}}
\hfil
\subfloat{\includegraphics[width=0.4\textwidth]{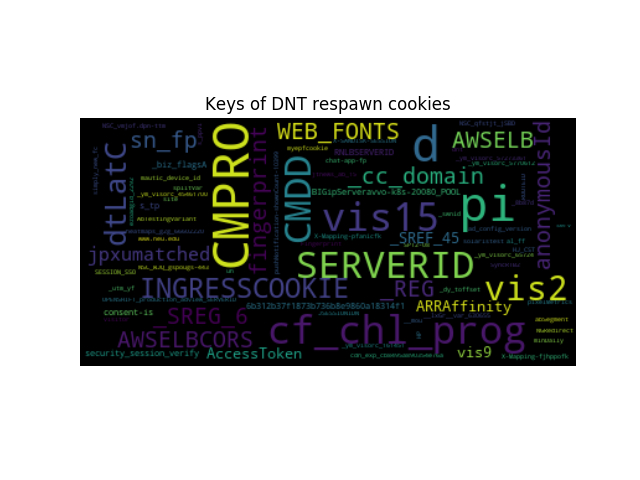}\label{fig:h}}
\caption{Keys of respawn cookies per feature}
    \label{fig:myfigure}
    \end{figure}

\subsection{Session feature analysis}
A session cookie get deleted when the user close her browser.
Unlike session cookies where no expiration date is associated to the cookie, 
persistent cookies have an expiration date and are get deleted within this last.

\begin{figure}[!htbp]
    \centering
    \includegraphics[width=0.4\textwidth]{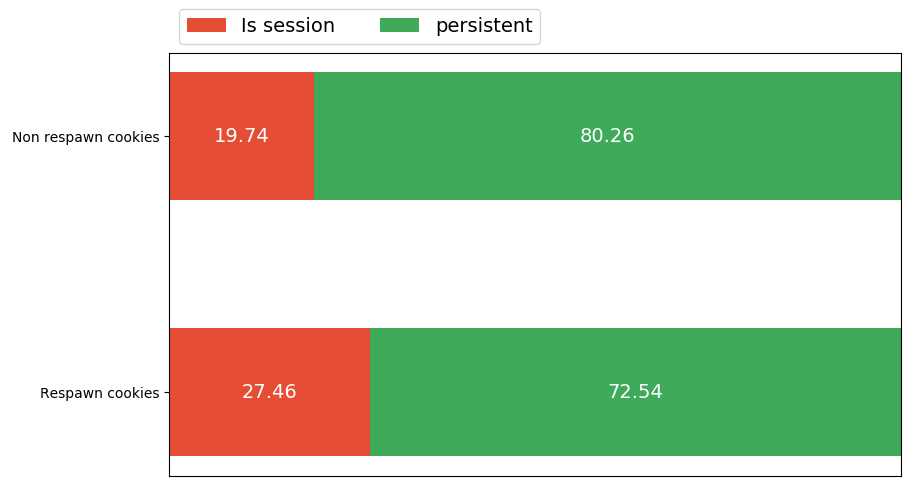}
    \caption{Percentage of usage of session cookies in respawned and non respawned cookies. }
    \label{fig:session}
\end{figure}

Figure \ref{fig:session} present the percentage of session and persistent cookies among \textit{respawn} and \textit{non respawn} cookies.
From the figure we see that 27.46\% of respawned cookies are session cookies compared to 19.74\% of \textit{non respawned cookies}.

\subsection{Crawling methodology}
Our goal is to compare different crawling algorithms. We use a set of $100$ sites for this experiment. In the following we describe the two studied crawling algorithms.
%\NB{Style: don't finish a section with ":". }
%\IF{Ok}

\subsubsection{Sequential crawling}
For every site \textit{site} we:
\begin{itemize}
    \item We perform a statless crawling instance as described in Section \ref{sec:methodology}  from machine1 :  \textit{$crawl_{1}$}
    \item We perform a statless crawling instance from machine2 to detect machine unrelated cookies \textit{$crawl_{3}$}
    %\NB{What is machine2? You introduced only one machine in Table 3 above... Not clear.}
    %\IF{I Added machine 2 to the table}
    \NB{Why machine 2 has crawl 3? it's confusing...}
    \item We perform a second statless crawling instance from machine1 \textit{$crawl_{2}$}
    \item if respawning detected in \textit{site}
    \begin{itemize}
    \item  \textit{for \textit{f} in features:}
    \begin{itemize}
 
          \item We spoof \textit{f}
        \item We perform statless crawling instance  of \textit{site}.
   \end{itemize} 
   \item we perform a control crawl
   \end{itemize} 
\end{itemize}

\begin{figure}[!h]
    \centering
    \includegraphics[width=0.70\textwidth]{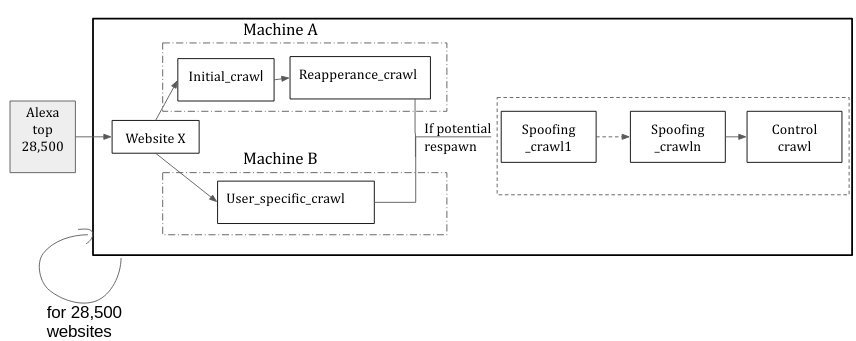}
    \caption{Sequential crawling of k sites \textit{For every site in k we perform (1)  an initial crawl $crawl_1$ from machine 1 and, (2) we start  a remote crawl $crawl_3$ from machine 2 to detect machine unrelated cookies. (3) after $crawl_1$ finishes we start $crawl_2$ from machine 1 to detect cookies reappearance. (4) using $crawl_1$,  $crawl_2$ and $crawl_3$ we check if we detect potential respawning in the site (the site contains a cookies that reappears in $crawl_2$ and is not machine unrelated) if it's the case, we (5) spoof one feature at time and perform a craw ($crawl_4$ ... $crawl_n$ with n is the number of studied features). Finally (6) we perform a control crawl.}}
    \label{fig:seq}
\end{figure}

The goal is to crawl 100 websites. 
In this experiment (Figure \ref{fig:seq}) we used one browser instance.
For every round, using this browser, we visit one site.
We analyzed two features (user agent, and geolocation).

%\textbf{Crawling 100 sites using sequential approach took 6h 40 min}
\textbf{Crawling 100 sites using sequential approach took 3h 54 min}

\begin{table}[!h]
    \centering
    \begin{tabular}{|p{5 cm}| p {3 cm}|p {3 cm}|}
    \hline
        \textbf{Task} & \textbf{Sequential execution time } & \textbf{Hybrid execution time}  \\ \hline
         crawl1 \& crawl 2 & 9,534 s & 6,820 s \\ \hline
         Synchronization with remote crawl & 709 s  & 3 s\\ \hline
         Processing & 123 s & 2 s \\ \hline
         Feature spoofing crawls & 2,380 s & 1,278 s \\ \hline
         \textbf{Total execution time} & 12,746 s & 8,103 s \\ \hline
    \end{tabular}
    \caption{Execution time of sequential  and hybrid crawling. \textit{\textit{Processing}: We extract the set of respawned websites (In total we detect 17 respawned sites in  sequential while we detect 19 in hybrid). \textit{Feature spoofing crawls}: we perform three crawls at this step ($crawl_4$ with spoofed geolocation, $crawl_5$ with spoofed UA and a control crawl). }}
    \label{tab:timer}
\end{table}{}

\begin{table}[]
    \centering
    \begin{tabular}{|p {4 cm}| p {4 cm} | p {4 cm} |p {4 cm} |}
    \hline
         & \textbf{$Crawl_1$\& $Crawl_2$} & \textbf{Feature spoofing crawls} & \textbf{Total}    \\ \hline
         \multicolumn{4}{c}{\textbf{Sequential crawling}}\\ \hline
        \textbf{Initiation}  &  3,542 s & 947 s & 4,489 s \\ \hline
        \textbf{Crawling} &  5,804 s & 1,353 s &  7,157 s  \\ \hline
         \multicolumn{4}{c}{\textbf{Hybrid crawling}}\\ \hline
        \textbf{Initiation}  & 5  s & 6 s & 11 s \\ \hline
        \textbf{Crawling} &  6,812 s & 1,269 s &  8,081 s  \\ \hline
    \end{tabular}
    \caption{Description of crawls execution time.\textit{ We have two main steps (1) Initiation: We update the task manager and the browser configuration. (2) Crawling: We visit Alexa top 100 websites.}}
    \label{tab:timerdescription}
\end{table}{}

\begin{table}[!h]
    \centering
    \begin{tabular}{|p{5 cm}| p {3 cm}|}
    \hline
        \textbf{Task} & \textbf{Sequential execution time }  \\ \hline
         crawl1 \& crawl 2 & 8,796 s  \\ \hline
         Synchronization with remote crawl & 433 s  \\ \hline
         Processing & 119 s  \\ \hline
         Feature spoofing & 2,612 \\ \hline
         \textbf{Total execution time} & 11,960 s \\ \hline
    \end{tabular}
    \caption{Execution time of sequential crawling after improvement. \textit{Initiation of $Crawl_1$\& $Crawl_2$ is reduced to 2,477 s}}
    \label{tab:timer}
\end{table}{}

\iffalse
\NB{In all these experiments, do you always target the same 500 sites?}
%we use multiple browsers in parallel.

The goal is to crawl 100 websites. We split 100 websites into 5 groups, of 20 websites each.

In this experiment we used 5 browsers.
For every round, using these browsers, we visit 5 websites in parallel in $crawl_1$, $crawl_2$ and $crawl_3$. 
\NB{I don't get it. how many  sites per browser were crawled?}
We then analyze the 5 websites and extract those where we detect potential respawning $Set_{\mathit{respawn\_sites}}$.
We continue the analysis by only crawling sites in  $Set_{\mathit{respawn\_sites}}$. 
\NB{how many features were analysed?}

The number of parallel browsers used in $crawl_4$ ... $crawl_n$ and $controlCraw$ is equal to the number of sites in $Set_{\mathit{respawn\_sites}}$.

\begin{itemize}
    \item Execution time: 2h50min
\end{itemize}

%The 5 browsers were used in 
%in this study we used 5 browsers in crawl1, crawl2 and crawl3. Starting from crawl4 we launch browsers with the 
%Browsers on hold.
\begin{itemize}
    \item + No delay between site visit in different modes.
    \item - Slower
    \NB{than what?}
\end{itemize}
\fi

\subsubsection{Hybrid crawling}
We split visited sites to 100, for every 100 sites we perform same steps as in hybrid.

%\begin{itemize}
%    \item Execution time: 1h20min
%\end{itemize}

\begin{figure}[!h]
    \centering
    \includegraphics[width=0.70\textwidth]{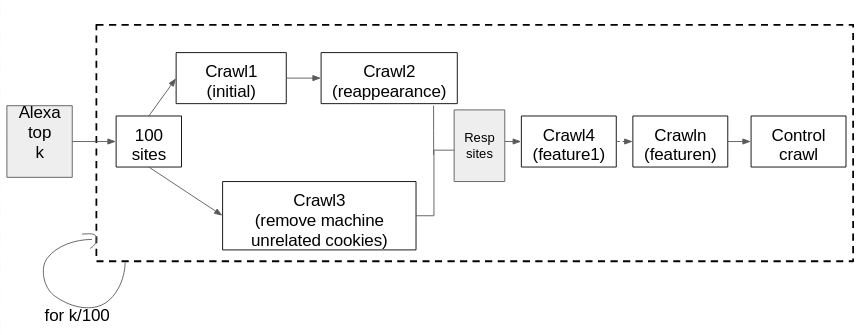}
    \caption{Hybrid crawling. \textit{We split k visited sites to 100, and for every group of 100 sites we perform same steps described in Figure \ref{fig:seq}} }
    \label{fig:hybrid}
\end{figure}

%\NB{Assign a unique label to each figure in order to refere to them in the text. }

Using the hybrid approach (Figure \ref{fig:hybrid}) we ensure a shorter delay between the \textit{site} visits compared to block crawling and a shorter execution time compared to hybrid crawling.

%\textbf{Crawling 100 sites using this approach took 3h 20 min}

\textbf{Crawling 100 sites using this approach took 2h 25 min}

\begin{table*}[!h]
  \centering
  \begin{tabular}{ | p{.65cm} | c  | c | p {.5cm} |}
    \hline
    &  Session & Persistent  & \\ \hline
        \begin{turn}{90}First-Party\end{turn}
 
    & 
    \begin{minipage}{.4\textwidth}
      \includegraphics[width=\linewidth]{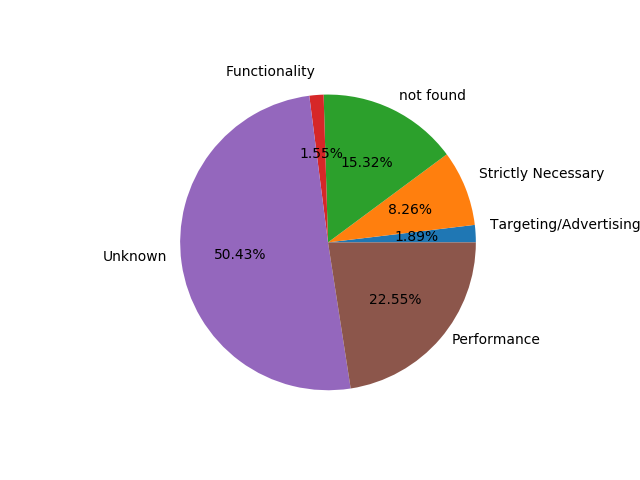}
      \caption*{ 368 (19.54\%) cookies}
    \end{minipage}
    &
    \begin{minipage}{.4\textwidth}
      \includegraphics[width=\linewidth  ]{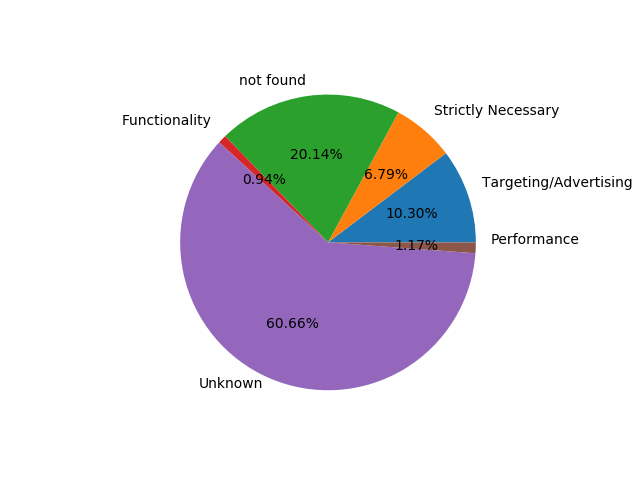}
      \caption*{640 (33.90\%) cookies}
    \end{minipage}
    & 
    \begin{turn}{90}1008 (53.53\%)\end{turn}

    \\ \hline
    
    \begin{turn}{90}Third-Party\end{turn}
    & 
    \begin{minipage}{.4\textwidth}
      \includegraphics[width=\linewidth]{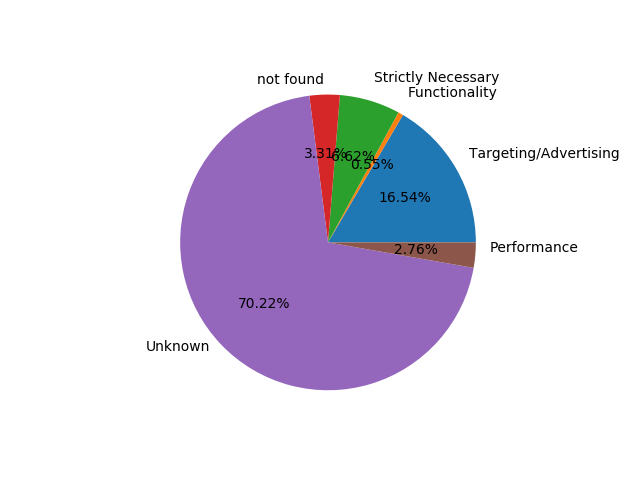}
      \caption*{97 (5.15\%) cookies}
    \end{minipage}
    
    &
    \begin{minipage}{.4\textwidth}
      \includegraphics[width=\linewidth]{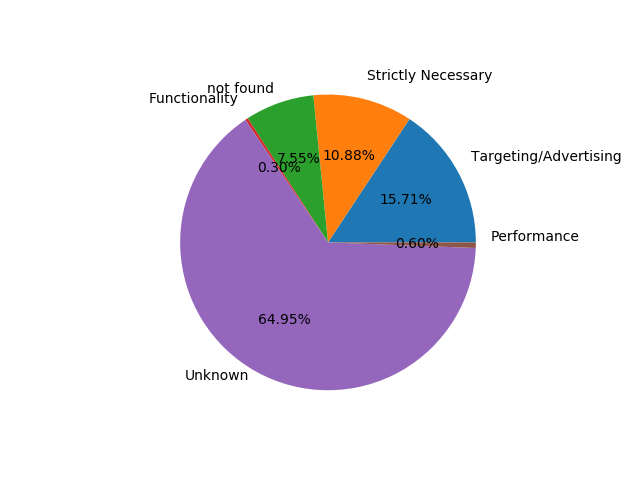}
      \caption*{778 (41.32\%) cookies}
    \end{minipage}
    & 
     \begin{turn}{90}875 (46.47\%)\end{turn}

    \\ \hline
    Total & 465 (24.69\%) &  1,418 (75.31\%) &  
            \begin{turn}{45}1883\end{turn}
  
    \\ \hline
  \end{tabular}
  \caption{Overview of respawned cookies characteristics}\label{tab:overview_resp}
\end{table*}
